# Supplementary material for: Tight Bounds for Sampling q-Colorings via Coupling from the Past
Source: arXiv:2511.04982 source file (2025-11-19)
Supplement: Supplementary file 1 [file appendixA.tex]

\section{Proof of conversion step under \texorpdfstring{$q > (2.5 + \eta)\Delta$}{q > (2.5 + η)Δ}}
\label{appendix:A}

\begin{lemma}
    Assume $q \ge (2.5 + \eta)\Delta$ for some constant $\eta > 0$. Then, for each vertex $v \in V \setminus S$, there exists a way to construct the color set $A \subseteq [q]$ of size $\Delta$—depending only on the current bounding list $\mathcal{L}$—such that after applying \textsc{Compress} updates to all unmarked neighbors of $v$, the effective constraint set for $v$ satisfies:
    $$
    \abs\slv - \frac{1}{2}\abs\dlv < (1.5 + \eta)\Delta,
    $$
    which suffices to guarantee the success of the subsequent \textsc{Disjoint} update on $v$.
\end{lemma}

\begin{proof}
    Fix a vertex $v \in V \setminus S$ and let $\Gamma(v)$ denote its neighbors. Let $x$ be the number of neighboring bounding sets not contained in $\dlv$, and let $y$ be the number of bounding sets that are in $\dlv$. By definition, we have $x + y \le \Delta$ and $x + y \ge \left(\frac{1}{2} - \eta\right)\Delta$.
    
    We now choose a color set $A$ of size $\Delta$ to minimize the expression $\abs\slv - \frac{1}{2}\abs\dlv$. Suppose $A$ include $a$ bounding sets from outside $\dlv$ and $b$ bounding sets from inside $\dlv$. Then we can upper bound:
    \[
    \abs\slv - \frac{1}{2}\abs\dlv \le (1 - x - y) + 1.5x + y + (1 - 1.5a - 2b),
    \]
    which arises by adding the baseline contribution from all bounding sets, plus the worst-case addition from new bounding sets brought into $\slv$ through \textsc{Compress}. This reduces to the following optimization problem:
    \begin{align*}
        \max_{x, y} \min_{a, b} \quad & (1 - x - y) + 1.5x + y + (1 - 1.5a - 2b) \\
        \text{subject to} \quad & \left(\frac{1}{2} - \eta\right)\Delta \le x + y \le \Delta, \\
        & a \le x,\quad b \le y, \\
        & 1.5a + 2b \le \Delta,\\
        & a,b,x,y \in \mathbb{N}.
    \end{align*}

    Since this is an integer program over a constant number of variables, we may relax it to a linear program with continuous variables, incurring at most an additive $O(1)$ loss in the objective. We normalize all quantities by $\Delta$, so $x, y, a, b$ now denote fractions in $[0,1]$:
    \begin{align*}
    \max_{x, y} \min_{a, b} \quad & 2+0.5x-1.5a-2b \\
    \text{subject to} \quad & \frac{1}{2} - \eta \le x + y \le 1, \\
    & 1.5a + 2b \le 1,\\
    & \quad 0 \le a \le x\le 1,\quad 0 \le b \le y\le 1, \\
    \end{align*}

    For fixed $x,y$ the inner minimisation over $a,b$ is equivalent to maximising $1.5a+2b$. The maximum of $1.5a+2b$ under these bounds is $M(x,y)=\min(1,1.5x+2y)$. Hence the outer problem becomes
    \begin{align*}
    \max_{x,y}\quad&G(x,y)=2+0.5x-\min(1,1.5x+2y)\\
    \text{subject to}\quad& 0.5-\eta\le x+y\le 1,\\
    &0\le x,y\le 1.
    \end{align*}
    
    We analyze two cases:

    \textbf{Case 1:} If $1.5x + 2y \le 1$, then $G(x,y) = 2 - x - 2y$, which is strictly decreasing in both $x$ and $y$. Since $x + y \ge 0.5 - \eta$, the maximum occurs at $x = 0.5 - \eta$, $y = 0$, yielding $G = 2 - (0.5 - \eta) = 1.5 + \eta$.

    \textbf{Case 2:} If $1.5x + 2y \ge 1$, then $M(x,y) = 1$, so $G(x,y) = 1 + 0.5x$, which is increasing in $x$. The maximum occurs at $x = 1$, $y = 0$, giving $G = 1.5$.

    In both cases, we have $G(x,y) \le 1.5 + \eta$, completing the proof.

\end{proof}
